# Supplementary material for: P-MOSS: Scheduling Main-Memory Indexes Over NUMA Servers Using Next Token Prediction
Source: arXiv:2411.02933 source file (2026-01-21)
Supplement: Supplementary file 1 [file Appendix.tex]

% \balance{}

\section{Mapping Hardware PMU Statistics in \sys{}}
Different hardware platforms can use the same or different event names to profile a particular hardware event. Hence, a mapping is required to align platform-specific events to the featurization format proposed in \sys{}. Table~\ref{tab:pmu} gives the mapping of the core PMU statistics for the six servers on which \sys{} has been evaluated on. We use the Libpfm4~\cite{libpfm4} library to collect the raw Hexadecimal code of the hardware performance events. These events are then profiled using a C++ wrapper for Linux Perf Event API~\cite{perf}. To profile the off-core hardware statistics on Intel servers, \sys{} integrates Intel PCM~\cite{pcm} in it's runtime system. For each NUMA socket, it collects per-channel memory read and write bandwidths, and the data traffic per each incoming Ultra Path Interconnects (UPI, for short) link. 
\begin{small}
	\begin{table*}[t]
    \setlength{\abovecaptionskip}{-0.3pt}
	\caption{The profiled hardware performance events in \sys{}.}
		\label{tab:pmu}
		\centering
  \small
		\begin{tabular}{l|l|l|l|l|l|l}
          \hline
		    \multirow{2}{*}
            {
            \makecell[l]{
            HW 
            \\
            % Component 
            }
            } & &
            \multicolumn{5}{c}{Machines}\\
            \cline{2-7}
             & Event & AMD Milan:1NPS, 4NPS & Intel Skylake X & Intel Sandy Bridge & NVIDIA Grace Hopper & IBM Power\\
			\hline \hline
            
            \multirow{4}{*}
            {
            {\rotatebox{90}{\parbox[c]{1cm}{\centering Front End}}}
            } 
            & CPU Cycles & \multicolumn{5}{c}{\texttt{PERF\_COUNT\_HW\_CPU\_CYCLES}} \\
            \cline{2-7}
			& Instructions & \multicolumn{5}{c}{\texttt{PERF\_COUNT\_HW\_INSTRUCTIONS}} \\
            \cline{2-7}
            & L1-I Miss& \multicolumn{4}{c|}{\texttt{PERF\_COUNT\_HW\_CACHE\_L1I:READ:MISS}} & \texttt{x}\\
            \cline{2-7}
            & Brach Miss& \multicolumn{4}{c|}{\texttt{PERF\_COUNT\_HW\_BRANCH\_MISSES}} & \texttt{x}\\
            \cline{2-7}
            \hline 
            \multirow{5}{*}{
            {\rotatebox{90}{\parbox[c]{3cm}{\centering Cache Sub-system}}}
            } 
            & L1-D Miss & \multicolumn{4}{c|}{\texttt{PERF\_COUNT\_HW\_CACHE\_L1D:READ:MISS}} 
            & \texttt{x}
            \\
            \cline{2-7}
			
            & LL Miss 
            & \makecell[l]
            {
            \texttt{DEMAND\_DATA\_CACHE\_}\\\texttt{FILLS\_FROM\_SYSTEM}\\
            \texttt{:EXT\_CACHE\_LCL}
            } 
            & \multicolumn{2}{c|}{
            \makecell[l]
            {\texttt{PERF\_COUNT\_HW\_CACHE\_LL:READ:MISS}
            % \\\texttt{}
            } 
            } 
            & \makecell[l]{\texttt{REQUESTS\_TO\_L2\_GROUP1:}\\\texttt{RD\_BLK\_X}} 
            & \makecell[l]
            {
            \texttt{PERF\_COUNT\_HW\_}\\
            \texttt{CACHE\_LL:}\\
            \texttt{READ:MISS}
            }
            \\
            \cline{2-7}
            
			& DTLB Miss
            & \multicolumn{4}{c|}{\texttt{PERF\_COUNT\_HW\_CACHE\_DTLB:READ:MISS}}
            & \texttt{x}\\
            \cline{2-7}
            
            & LL Write Miss
            & \makecell[l]
            {
                \texttt{REQUESTS\_TO\_L2\_}\\
                \texttt{GROUP1:RD\_BLK\_X}
            } 
            & \multicolumn{2}{c|}
            {
            \makecell[l]
            {
                \texttt{PERF\_COUNT\_HW}\\\texttt{\_CACHE\_LL:WRITE:MISS}
            }   
            } 
            &
            \makecell[l]{\texttt{LLC\_STORE\_MISSES}} 
            &
            \texttt{x}\\
            \cline{2-7}
            
            & \makecell[l]{L1-D/LL\\{Miss Latency }} 
            & 
            \makecell[l]{\texttt{UNC\_L3\_MISS\_LATENCY}} 
            & 
            \makecell[l]{\texttt{CYCLE\_ACTIVITY.}\\
            \texttt{CYCLES\_L3\_MISS}
            }
            & 
            \makecell[l]{\texttt{CYCLE\_ACTIVITY:}\\
            \texttt{CYCLES\_L1D\_}\\
            \texttt{PENDING}
            }
            &
            \makecell[l]{\texttt{STALL\_BACKEND\_MEM}
            } 
            & 
            \makecell[l]
            {
            \texttt{PM\_CMPLU\_}\\
            \texttt{STALL\_DMISS\_}\\
            \texttt{LMEM}
            } 
            \\
            \hline
            \multirow{6}{*}{
            {
            \rotatebox{90}{\parbox[c]{5cm}{\centering Memory Sub-system}}}
            } 
            & Memory Access 
            & \makecell[l]{
            \texttt{DEMAND\_DATA\_CACHE\_}\\\texttt{FILLS\_FROM\_SYSTEM}\\
            \texttt{INT\_CACHE}
            } 
            &\multicolumn{2}{c|}
            {
            \makecell[l]{
            \texttt{PERF\_COUNT\_HW}\\
            \texttt{\_CACHE\_NODE:READ:ACCESS}
            } 
            } 
            &
            \makecell[l]{
            \texttt{MEM\_ACCESS\_RD}
            } 
            & 
            \makecell[l]
            {
            \texttt{PM\_DATA\_}\\
            \texttt{ALL\_FROM\_ON\_}\\
            \texttt{CHIP\_CACHE}
            } 
            \\
            \cline{2-7}
            
			& Memory Miss
            & \makecell[l]
            {
            \texttt{DEMAND\_DATA\_CACHE\_}\\\texttt{FILLS\_FROM\_SYSTEM}\\
            \texttt{:EXT\_CACHE\_RMT}
            } 
            & \multicolumn{2}{c|}
            {
                \makecell[l]{
                \texttt{PERF\_COUNT\_HW}\\
                \texttt{\_CACHE\_NODE:READ:MISS}} 
            }
            &
            \makecell[l]{\texttt{BUS\_ACCESS}}
            & 
            \makecell[l]
            {
            \texttt{PM\_DATA\_}\\
            \texttt{ALL\_FROM\_OFF\_}\\
            \texttt{CHIP\_CACHE}
            } 
            \\
            \cline{2-7}
			
            & \makecell[l]{
            Memory Write\\
            Miss
            } 
            & \multicolumn{3}{c|}
            {
            \texttt{PERF\_COUNT\_HW\_CACHE\_NODE:WRITE:MISS}
            } 
            & 
            \texttt{MEM\_ACCESS\_WR}
            & \texttt{x}
            \\
            \cline{2-7}
            
            & \makecell[l]{
            Memory Miss\\
            Latency
            } 
            & 
            \makecell[l]
            {\texttt{CYCLES\_NOT\_IN\_HALT}
            } 
            & 
            \makecell[l]
            {
            \texttt{CYCLE\_ACTIVITY.}\\
            \texttt{CYCLES\_MEM\_ANY}
            }
            &
            \makecell[l]{\texttt{CYCLE\_ACTIVITY:}\\
            \texttt{CYCLES\_L2\_}\\
            \texttt{PENDING}
            }
            &
            \makecell[l]{\texttt{STALL\_BACKEND\_MEM}
            } 
            & \makecell[l]
            {
            \texttt{PM\_CMPLU\_}\\
            \texttt{STALL\_DMISS\_}\\
            \texttt{REMOTE}}
            \\
            \cline{2-7}
            & 
            \makecell[l]
            {
            Local DRAM\\
            Access
            }
            & \makecell[l]
            {
            \texttt{DEMAND\_DATA\_CACHE\_}\\
            \texttt{FILLS\_FROM\_SYSTEM}\\
            \texttt{MEM\_IO\_LCL}
            } 
            & 
            \makecell[l]{\texttt{MEM\_LOAD\_L3\_MISS}\\
            \texttt{\_RETIRED}\\
            \texttt{LOCAL\_DRAM}}
            &
            \makecell[l]
            {
            \texttt{MEM\_LOAD\_UOPS\_}\\
            \texttt{LLC\_MISS\_RETIRED.}\\
            \texttt{LOCAL\_DRAM}
            }
            & 
            \makecell[l]{\texttt{L1D\_CACHE\_}\\\texttt{LMISS\_RD}} 
            &
            \makecell[l]{
            \texttt{PM\_DATA\_ALL}\\\texttt{\_FROM\_LMEM}
            }            
            \\
            \cline{2-7}
            
            & \makecell[l]{
            Remote DRAM\\
            Access
            }
            & \makecell[l]{\texttt{DEMAND\_DATA\_CACHE\_}\\\texttt{FILLS\_FROM\_SYSTEM}\\
            \texttt{MEM\_IO\_RMT}
            } 
            & 
           
            \makecell[l]{
            \texttt{MEM\_LOAD\_L3\_MISS\_}\\
            \texttt{RETIRED\_}\\
            \texttt{:REMOTE\_DRAM}
            }
            &
            \makecell[l]
            {
            \texttt{MEM\_LOAD\_UOPS\_}\\
            \texttt{LLC\_MISS\_RETIRED.}\\
            \texttt{REMOTE\_DRAM}
            }
            &
            \makecell[l]{\texttt{L2D\_CACHE\_}\\\texttt{LMISS\_RD}} 
            & 
            \makecell[l]{\texttt{PM\_DATA\_ALL\_}\\\texttt{FROM\_DMEM}}
            
            \\
            \hline
		\end{tabular}
	\end{table*}
\end{small}

\section{Offline Dataset Composition in \sys{}}
During the training phase, \sys{} trains the DT on an offline dataset. The offline dataset comprises a diverse set of scheduling policies on different hardware architectures and query workload patterns. The offline dataset contains 7518 scheduling policies across five different hardware, and six different query workload patterns. Each scheduling policy includes seven samples in the offline dataset. 
About 14.63\%, 12.75\%, 1.76\%, and 71.03\% of these scheduling policies stem from the Grouped, Mixed, Spread and Random SN:T strategies, respectively. Tables~\ref{tab:offline_data_wk} and~\ref{tab:offline_data_sched} detail the offline dataset composition in \sys{}. 

\begin{small}
	\begin{table*}[htbp]
    \setlength{\abovecaptionskip}{-0.3pt}
    \caption{Breakdown of the Offline Dataset in terms of query workload and hardware.}
    \label{tab:offline_data_wk}
    \centering
    \begin{tabular}{l|l|l|l|l|l}
    \hline
    Workload 
    & \makecell[l]{
    \texttt{AMD Milan:1NPS}\\
      18.25\%
    } 
    & \makecell[l]{
    \texttt{AMD Milan:4NPS}\\
      24.21\%
    } 
    & 
    \makecell[l]{
    \texttt{Intel Skylake X }\\
      19.83\%
    } 
    &
    \makecell[l]{
    \texttt{Intel Sandy Bridge}\\
      23.09\%
    }
    &
    \makecell[l]{
    \texttt{NVIDIA Grace Hopper}\\
      14.62\%
    }\\
    \hline 
    \hline 
    50\% Read - 50\% Write & 2.86\% & 2.96\% & 3.75\% & 2.86\% & 3.16\% \\
    100\% Read & 5.03\% & 4.83\% & 4.44\% & 5.23\% & 2.96\% \\
    95\% Scan - 5\% Insert & 2.56\% & 5.03\% & 3.94\% & 2.76\% & 1.97\% \\
    100\% Scan & 4.44\% & 3.55\% & 2.86\% & 4.14\% & 3.06\% \\
    20\% Read - 30\% Scan - 50\% Insert & 2.17\% & 4.73\% & 3.16\% & 4.64\% & 2.17\% \\
    25\% Read - 50\% Scan - 25\% Insert  & 2.17\% & 4.64\% & 2.86\% & 4.83\% & 2.17\% \\
    \hline
    \end{tabular}
	\end{table*}
\end{small}

\begin{small}
\begin{table*}[htbp]
    \setlength{\abovecaptionskip}{-0.3pt}
    \caption{Breakdown of the Offline Dataset in terms of the heuristic scheduling policies and hardware.}
    \label{tab:offline_data_sched}
    \centering
    \begin{tabular}{l|l|l|l|l|l}
    \hline
    \makecell[l]{
    SN:T Scheduling\\
      Policy
    } 
    & \makecell[l]{
    \texttt{AMD Milan:1NPS}\\
      18.25\%
    } 
    & \makecell[l]{
    \texttt{AMD Milan:4NPS}\\
      24.21\%
    } 
    & 
    \makecell[l]{
    \texttt{Intel Skylake X }\\
      19.83\%
    } 
    &
    \makecell[l]{
    \texttt{Intel Sandy Bridge}\\
      23.09\%
    }
    &
    \makecell[l]{
    \texttt{NVIDIA Grace Hopper}\\
      14.62\%
    }\\
    \hline
    \hline
    Grouped & 2.70\% & 3.17\% & 2.33\% & 3.45\% & 2.98\% \\
    Mixed & 3.07\% & 3.72\% & 1.86\% & 3.91\% & 0.19\% \\
    Spread & 0.28\% & 0.74\% & 0.09\% & 0.65\% & 0.00\% \\
    Random & 12.20\% & 16.57\% & 15.55\% & 15.08\% & 11.45\% \\
    \end{tabular}
\end{table*}
\end{small}

\section{Learned schedules in \sys{}}
\Cref{fig:exp_0,fig:exp_1,fig:exp_2,fig:exp_3} give the learned schedules of \sys{} for YCSB read-write, point lookup, scan and mixed workload, respectively. Figure~\ref{fig:exp_4} gives the learned schedules of \sys{} in unseen environment. 
Figure~\ref{fig:baseline} gives the representative scheduling policies of four SN:T baselines: Grouped, Mixed, Spread, and Random. The Core IDs are randomly generated. Each grid cell represents an index slice. The text inside each grid cell denotes the `Core ID', where the query for the corresponding index slice is scheduled. Same colored grid cells indicate the corresponding index slices are scheduled on the same NUMA node.

\begin{figure*}[t]
    % \captionsetup{belowskip=-12pt}
    \captionsetup{aboveskip=-0.5pt}
    \centering
    \includegraphics[width=0.70\textwidth]{figures/exp_0.pdf}
    \caption{
    % Learned schedules of \sys{} for 
    YCSB Read-Write workload.
    }
    \label{fig:exp_0}
    \includegraphics[width=0.70\textwidth]{figures/exp_1.pdf}
    \caption{
    % Learned schedules of \sys{} for 
    YCSB Lookup workload.}
    \label{fig:exp_1}
    \includegraphics[width=0.70\textwidth]{figures/exp_2.pdf}
    \caption{
    % Learned schedules of \sys{} for 
    YCSB Scan workload.}
    \label{fig:exp_2}
    \includegraphics[width=0.70\textwidth]{figures/exp_3.pdf}
    \caption{
    % Learned schedules of \sys{} for 
    YCSB Mixed workload.}
    \label{fig:exp_3}
        \includegraphics[width=0.70\textwidth]{figures/exp_4.pdf}
    \caption{
    % Learned schedules of \sys{} in 
    Unseen environment.}
    \label{fig:exp_4}
        \includegraphics[width=0.70\textwidth]{figures/baseline.pdf}
    \caption{
    % Learned schedules of \sys{} for 
    SN:T baselines.}
    \label{fig:baseline}
\end{figure*}
